# Supplementary material for: Local and global densities for Weierstrass models of elliptic curves
Source: arXiv:2003.08454 ancillary file (2021-10-18)
Supplement: Supplementary file 1 [file Weierstrass_counts.pdf]

# Weierstrass\_counts

October 18, 2021

## 1 Checking the distribution of discriminant valuations of Weierstrass models with additive reduction at $p = 2$ or $p = 3$

```
[1]: from sage.schemes.elliptic_curves.kodaira_symbol import KodairaSymbol
      from collections import Counter
```

Function for counting the occurrences of different discriminant valuation  $n$  for a given Kodaira type at a give prime for a range o conductors in the database:

```
[2]: def disc_val_count(ks, pr=2, Nmax=1000):
      c = Counter()
      KS = KodairaSymbol(ks)
      for N in srange(11, Nmax):
          if N%pr^2:
              continue
          for E in cremona_curves([N]):
              if E.kodaira_symbol(pr)==KS:
                  n = E.discriminant().valuation(pr)
                  c[n] += 1
      return c
```

Function to find one example of a given discriminant valuation for given Kodaira type and prime:

```
[3]: def find_one(ks, n, pr, Nmax=1000):
      KS = KodairaSymbol(ks)
      for E in cremona_curves(srange(11,Nmax)):
          if E.kodaira_symbol(pr)==KS and E.discriminant().valuation(pr)==n:
              return E.label()
```

### 1.1 Distribution for $p = 2$

$n = 4, 6, 7$  for Type II at 2:

```
[4]: disc_val_count("II", 2)
```

```
[4]: Counter({4: 67, 6: 30, 7: 12})
```

First curve with  $n = 4, 6, 7$  and Type II at 2:

```
[5]: [find_one("II", n, 2) for n in [4,6,7]]
```

```
[5]: ['48a4', '64a4', '128b2']
```

**$n = 11, 12, 14$  for Type II\* at 2:**

```
[6]: disc_val_count("II*", 2)
```

```
[6]: Counter({11: 89, 12: 23, 14: 6})
```

**First curve with  $n = 11, 12, 14$  and Type II\* at 2:**

```
[7]: [find_one("II*", n, 2) for n in [11, 12, 14]]
```

```
[7]: ['24a5', '176b1', '704d1']
```

**$n = 4, 6, 8, 9$  for Type III at 2:**

```
[8]: disc_val_count("III", 2)
```

```
[8]: Counter({4: 82, 6: 39, 9: 16, 8: 12})
```

**First curve with  $n = 4, 6, 8, 9$  and Type III at 2:**

```
[9]: [find_one("III", n, 2) for n in [4, 6, 8, 9]]
```

```
[9]: ['24a4', '32a2', '128a1', '256a1']
```

**$n = 10, 12, 14, 15$  for Type III\* at 2:**

```
[10]: disc_val_count("III*", 2)
```

```
[10]: Counter({10: 125, 12: 18, 15: 16, 14: 12})
```

**First curve with  $n = 10, 12, 14, 15$  and Type III\* at 2:**

```
[11]: [find_one("III*", n, 2) for n in [10,12,14,15]]
```

```
[11]: ['24a2', '352a1', '128b1', '256a2']
```

**$n = 4$  for Type IV at 2:**

```
[12]: disc_val_count("IV", 2)
```

```
[12]: Counter({4: 166})
```

**First curve with  $n = 4$  and Type IV at 2:**

```
[13]: find_one("IV", 4, 2)
```

[13]: '20a2'

$n = 8$  for Type IV\* at 2:

```
[14]: disc_val_count("IV*", 2)
```

[14]: Counter({8: 238})

First curve with  $n = 8$  and Type IV\* at 2:

```
[15]: find_one("IV*", 8, 2)
```

[15]: '20a1'

$n = 8, 9, 10$  for Type I<sub>0</sub>\*:

```
[16]: disc_val_count("I0*", 2)
```

[16]: Counter({8: 87, 9: 56, 10: 18})

First curve with  $n = 8, 9, 10$  and Type I<sub>0</sub>\* at 2:

```
[17]: [find_one("I0*", n, 2) for n in [8, 9, 10]]
```

[17]: ['48a1', '32a3', '192c1']

$n = 8$  for Type I<sub>1</sub>\*,  $n = 10, 12, 13$  for Type I<sub>2</sub>\*,  $n = 11, 12$  for Type I<sub>3</sub>\*, and  $n = n + 8, n + 10$  for Type I<sub>m</sub>\* for  $m \geq 4$  at 2:

```
[18]: for m in range(1,15):  
    print("I*{:}: {}".format(m,disc_val_count("I{:}*".format(m), 2, 1000 if m<12_  
    ↪else 2000)))
```

I\*1: Counter({8: 116})  
I\*2: Counter({10: 50, 12: 20, 13: 12})  
I\*3: Counter({11: 42, 12: 35})  
I\*4: Counter({12: 48, 14: 22})  
I\*5: Counter({13: 37, 15: 32})  
I\*6: Counter({14: 25, 16: 22})  
I\*7: Counter({17: 24, 15: 20})  
I\*8: Counter({18: 16, 16: 11})  
I\*9: Counter({19: 10, 17: 9})  
I\*10: Counter({18: 10, 20: 4})  
I\*11: Counter({21: 8, 19: 2})  
I\*12: Counter({20: 14, 22: 6})  
I\*13: Counter({21: 12, 23: 8})  
I\*14: Counter({22: 11, 24: 6})

## 1.2 Distribution for $p = 3$

$n = 3, 4, 5$  for Type II at 3:

```
[19]: disc_val_count("II", 3)
```

```
[19]: Counter({3: 50, 4: 17, 5: 7})
```

First curve with  $n = 3, 4, 5$  and Type II at 2:

```
[20]: [find_one("II", n, 3) for n in [3, 4, 5]]
```

```
[20]: ['27a3', '162b1', '243a1']
```

$n = 11, 12, 13$  for Type II\* at 3:

```
[21]: disc_val_count("II*", 3)
```

```
[21]: Counter({11: 43, 12: 15, 13: 5})
```

First curve with  $n = 11, 12, 13$  and Type II\* at 3:

```
[22]: [find_one("II*", n, 3) for n in [11, 12, 13]]
```

```
[22]: ['27a2', '162b2', '243b2']
```

$n = 3$  for Type III at 3:

```
[23]: disc_val_count("III", 3)
```

```
[23]: Counter({3: 111})
```

First curve with  $n = 3$  and Type III at 3:

```
[24]: find_one("III", 3, 3)
```

```
[24]: '36a1'
```

$n = 9$  for Type III\*:

```
[25]: disc_val_count("III*", 3)
```

```
[25]: Counter({9: 111})
```

First curve with  $n = 9$  and Type III\* at 3:

```
[26]: find_one("III*", 9, 3)
```

```
[26]: '36a3'
```

$n = 5, 6, 7$  for Type IV at 3:

```
[27]: disc_val_count("IV", 3)
```

```
[27]: Counter({5: 43, 6: 15, 7: 5})
```

First curve with  $n = 5, 6, 7$  and Type IV at 3:

```
[28]: [find_one("IV", n, 3) for n in [5,6,7]]
```

```
[28]: ['27a4', '162a1', '243b1']
```

$n = 9, 10, 11$  for Type IV\* at 3:

```
[29]: disc_val_count("IV*", 3)
```

```
[29]: Counter({9: 50, 10: 17, 11: 7})
```

First curve with  $n = 9, 10, 11$  and Type IV\* at 3:

```
[30]: [find_one("IV*", n, 3) for n in [9, 10, 11]]
```

```
[30]: ['27a1', '162a2', '243a2']
```

$n = 6$  for Type I<sub>0</sub>\* at 3:

```
[31]: disc_val_count("I0*", 3)
```

```
[31]: Counter({6: 159})
```

First curve with  $n = 6$  and Type I<sub>0</sub>\* at 3:

```
[32]: find_one("I0*", 6, 3)
```

```
[32]: '99d1'
```

$n = m + 6$  for Type I<sub>m</sub>\* at 3 (all  $m \geq 1$ ):

```
[33]: for m in range(1,15):
        print("I*{}: {}".format(m,disc_val_count("I{}*".format(m), 3, 1000 if m<12_
        ↪else 2000)))
```

```
I*1: Counter({7: 135})
```

```
I*2: Counter({8: 100})
```

```
I*3: Counter({9: 45})
```

```
I*4: Counter({10: 70})
```

```
I*5: Counter({11: 23})
```

```
I*6: Counter({12: 22})
```

```
I*7: Counter({13: 10})
```

```
I*8: Counter({14: 29})
```

```
I*9: Counter({15: 1})  
I*10: Counter({16: 12})  
I*11: Counter({17: 3})  
I*12: Counter({18: 31})  
I*13: Counter({19: 4})  
I*14: Counter({20: 12})
```

[ ]:
