# Supplementary material for: Local and global densities for Weierstrass models of elliptic curves
Source: arXiv:2003.08454 ancillary file (2021-10-18)
Supplement: Supplementary file 2 [file Weierstrass_densities.pdf]

# Weierstrass\_densities

October 18, 2021

## 1 Worksheet for Section 5 of “Local and global densities for Weierstrass models of elliptic curves” by John Cremona and Mohammad Sadek

Claims made in the paper are established using an ‘assert’ statement to assert that an identity or congruence holds.

### 1.0.1 Define a polynomial ring in which to work:

We essentially work in  $\mathbb{Z}[a_1, a_2, a_3, a_4, a_6]$ . The variables  $a'_i$  (aid) will represent  $a_i/p^{v_i}$  for suitable  $v_i \geq 0$ ,  $p$  will be a generic prime and  $q$  a fixed power of  $p$  (used for Types  $I_m^*$ ), and the variables  $t, u, \dots$  are auxiliary variables.

```
[1]: R.<a1,a2,a3,a4,a6, a1d, a2d, a3d, a4d, a6d, p, q, t, u, v, w, y, z> = ZZ[]
```

### Define the generic elliptic curve, its discriminant and other invariants:

```
[2]: E = EllipticCurve([a1,a2,a3,a4,a6])
      b2, b4, b6, b8 = E.b_invariants()
      Delta = E.discriminant()
```

### Define utility functions to evaluate $\Delta$ and the $b_i$ on $W(v_1, v_2, v_3, v_4, v_6)$ .

```
[3]: def DD(v1,v2,v3,v4,v6, pr=p):
      return Delta(a1=pr^v1*a1d, a2=pr^v2*a2d, a3=pr^v3*a3d, a4=pr^v4*a4d,
      ↪a6=pr^v6*a6d,
      p=pr)

      def BB2(v1,v2,v3,v4,v6, pr=p):
          return b2(a1=pr^v1*a1d, a2=pr^v2*a2d, a3=pr^v3*a3d, a4=pr^v4*a4d,
          ↪a6=pr^v6*a6d,
          p=pr)

          def BB4(v1,v2,v3,v4,v6, pr=p):
              return b4(a1=pr^v1*a1d, a2=pr^v2*a2d, a3=pr^v3*a3d, a4=pr^v4*a4d,
              ↪a6=pr^v6*a6d,
              p=pr)
```

```

def BB6(v1,v2,v3,v4,v6, pr=p):
    return b6(a1=pr^v1*a1d, a2=pr^v2*a2d, a3=pr^v3*a3d, a4=pr^v4*a4d,
    ↪a6=pr^v6*a6d,
            p=pr)

def BB8(v1,v2,v3,v4,v6, pr=p):
    return b8(a1=pr^v1*a1d, a2=pr^v2*a2d, a3=pr^v3*a3d, a4=pr^v4*a4d,
    ↪a6=pr^v6*a6d,
            p=pr)

```

## 1.1 Type II, $W(1, 1, 1, 1, 1)$ with $v(a_6) = 1$

### 1.1.1 (1) Type II, $p \geq 5$ :

[4]: `D = DD(1,1,1,1,1)`

We have  $\Delta \equiv -2^4 3^3 a_6^2 = -2^4 3^3 p^2 a_6'^2 \pmod{p^3}$ , so  $n = v(\Delta) \geq 2$ , with equality for  $p \geq 5$  (using  $p \nmid a_6'$ ):

[5]: `assert (D + 2^4*3^3*p^2*a6d^2) % p^3 == 0`

### 1.1.2 (2) Type II, $p = 2$

[6]: `D = DD(1,1,1,1,1, pr=2)`

Now we have  $\Delta \equiv a_3^4 = 2^4 a_3'^4 \pmod{2^5}$ :

[7]: `assert (D - 2^4*a3d^4) % 2^5 == 0`

So  $n \geq 4$ , and  $n = 4 \iff 2 \nmid a_3' \iff v(a_3) = 1$ . Now we assume  $v(a_3) \geq 2$ :

[8]: `D = DD(1,1,2,1,1, pr=2)`

Now  $\Delta \equiv a_1^4 a_4^2 - 2^4 a_6^2 = 2^6 (a_1'^4 a_4'^2 - a_6'^2) \equiv 2^6 (a_1'^4 a_4'^2 - 1) \pmod{2^7}$ :

[9]: `assert (D - 2^6*(a1d^4*a4d^2-a6d^2)) % 2^7 == 0`

So  $n \geq 6$ , with  $n = 6 \iff 2 \mid a_1' a_4'$ .

Otherwise, we impose the additional conditions that  $a_1'$  and  $a_4'$  are both odd:

[10]: `D = D(a1d=2*u+1, a4d=2*v+1, a6d=2*w+1)`

Now  $\Delta \equiv 2^7 \pmod{2^8}$ , so  $n = 7$ :

[11]: `assert (D-2^7) % 2^8 == 0`

The relative probabilities of the cases  $n = 4$ ,  $n = 6$ , and  $n = 7$  are  $1/2$ ,  $(1/2)(3/4) = 3/8$  and  $(1/2)(1/4) = 1/8$  respectively.

### 1.1.3 (3) Type II, $p = 3$

[12]: `D = DD(1,1,1,1,1, pr=3)`

Now we have  $\Delta \equiv -a_4^3 = -3^3 a_4'^3 \pmod{3^4}$ :

[13]: `assert (D + 3^3*a4d^3) % 3^4 == 0`

Hence  $n \geq 3$ , with  $n = 3 \iff 3 \nmid a_4' \iff v(a_4) = 1$ . Assume  $v(a_4) \geq 2$ :

[14]: `D = DD(1,1,1,2,1, pr=3)`

Now  $\Delta \equiv -3a_2^2 a_6 \equiv -3^4 a_2'^2 a_6' \pmod{3^5}$ :

[15]: `assert (D + 3^4*a2d^2*a6d) % 3^5 == 0`

Hence  $n \geq 4$ , with  $n = 4 \iff 3 \nmid a_2' \iff v(a_2) = 1$  (since  $3 \nmid a_6'$ ). Assume that  $v(a_2) \geq 2$ :

[16]: `D = DD(1,2,1,2,1, pr=3)`

Now  $\Delta \equiv -3^3 a_6^2 = -3^5 a_6'^2 \pmod{3^6}$ , so  $n = 5$ :

[17]: `assert (D + 3^5*a6d^2) % 3^6 == 0`

The relative probabilities of the cases  $n = 3$ ,  $n = 4$ , and  $n = 5$  are  $2/3$ ,  $(1/3)(2/3) = 2/9$ , and  $(1/3)(1/3) = 1/9$  respectively.

## 1.2 Type III, $W(1, 1, 1, = 1, 2)$ with $v(a_4) = 1$

### 1.2.1 Type III, $p \neq 2$

[18]: `D = DD(1,1,1,1,2)`

Here,  $\Delta \equiv -2^6 a_4^3 = -2^6 p^3 a_4'^3 \pmod{p^4}$ :

[19]: `assert (D + 2^6*p^3*a4d^3) % p^4 == 0`

Hence  $n \geq 3$ , with  $n = 3$  exactly for  $p \neq 2$  (since  $p \nmid a_4'$ ).

### 1.2.2 Type III, $p = 2$

[20]: `D = DD(1,1,1,1,2, pr=2)`

Now,  $\Delta \equiv a_3^4 = 2^4 a_3'^4 \pmod{2^5}$ :

[21]: `assert (D - 2^4*a3d^4) % 2^5 == 0`

So  $n \geq 4$ , with  $n = 4 \iff p \nmid a_3' \iff v(a_3) = 1$ . Otherwise assume  $v(a_3) \geq 2$ :

[22]: `D = DD(1,1,2,1,2, pr=2)`

Now  $\Delta \equiv a_1^4 a_4^2 = 2^6 a_1^4 a_4^2 \equiv 2^6 a_1^4 \pmod{2^7}$ :

[23]: `assert (D - 2^6*a1d^4*a4d^2) % 2^7 == 0`

So  $n \geq 6$ , with  $n = 6 \iff v(a_1) = 1$ . Otherwise assume  $v(a_1) \geq 2$ :

[24]: `D = DD(2,1,2,1,2, pr=2)`

Now,  $\Delta \equiv 2^8(a_2^2 + a_3^4 + a_6^2) \pmod{2^9}$ , treating separately the cases  $a_6'$  even/odd

[25]: `assert all(((D - 2^8*(a2d^2*a4d^2+a3d^4+a6d^2))(a6d=2*w+r) % 2^9)==0 for r in [0,1])`

Hence  $n \geq 8$ , with equality if and only if  $a_2' + a_3' + a_6'$  is odd. To continue we set  $a_6' = a_2' + a_3' + 2w$ :

[26]: `D = D(a6d=a2d+a3d+2*w, a4d=2*u+1)`

We have  $n \geq 9$  (for  $a_3'$  even/odd):

[27]: `assert all((D(a3d=2*w+r)%2^9==0) for r in [0,1])`

Moreover,  $n = 9$  exactly, as we can see by considering  $\Delta \pmod{2^{10}}$ , considering the cases of even/odd  $a_3'$  separately:

[28]: `assert all(((D(a3d=2*w+r)-2^9)%2^10)==0 for r in [0,1])`

In summary, we have  $n = 4, 6, 8, 9$ , with relative probabilities  $1/2, 1/4, 1/8, 1/8$ .

### 1.3 Type IV, $W(1, 1, 1, 2, 2)$ with $v(b_6) = 2$

#### 1.3.1 Type IV, $p \neq 3$

[29]: `D = DD(1,1,1,2,2, p)`  
`B6 = BB6(1,1,1,2,2, p)`

Now we have  $\Delta \equiv -3^3 b_6^2 \pmod{p^5}$ , so  $n = 4$  when  $p \neq 3$ :

[30]: `assert (D + 3^3*B6^2) % p^5 == 0`

#### 1.3.2 Type IV, $p = 3$

[31]: `D = DD(1,1,1,2,2, pr=3)`  
`B6 = BB6(1,1,1,2,2, pr=3)`

Now we have  $\Delta \equiv -a_2^3 b_6 = -3^3 a_2^3 b_6 \pmod{3^6}$ :

[32]: `assert (D + 3^3*a2d^3*B6) % 3^6 == 0`

Hence  $n \geq 5$ , with  $n = 5 \iff 3 \nmid a_2'$ . Otherwise assume  $v(a_2) \geq 2$ :

[33]: `D = DD(1,2,1,2,2, pr=3)`

We now find that  $\Delta \equiv b_4^3 \pmod{3^7}$ :

[34]: `B4 = BB4(1, 2, 1, 2, 2, pr=3)`  
`assert (D-B4^3)%3^7 == 0`

Hence  $n \geq 6$ , with equality if and only if  $v(b_4) = 2$ , which is if and only if  $a'_4 \not\equiv a'_1 a'_3 \pmod{3}$ .  
 Otherwise we set  $a'_4 = a'_1 a'_3 + 3t$ :

[35]: `D = D(a4d=a1d*a3d+3*t)`

Now  $n = 7$  exactly, since  $\Delta \equiv -3^3 b_6^2 \pmod{3^8}$ :

[36]: `B6 = BB6(1,2,1,2,2, pr=3)`  
`assert (D+3^3*B6^2) % 3^8 == 0`

In summary,  $n = 5, 6, 7$  with relative probabilities  $2/3, 2/9, 1/9$ .

#### 1.4 Type $I_0^*$ , $W(1, 1, 2, 2, 3)$ with $\text{disc}(g) = 6$

[37]: `g = PolynomialRing(R, 'x')([a6,a4,a2,1])`  
`show(g)`

$$x^3 + a_2x^2 + a_4x + a_6$$

##### 1.4.1 Type $I_0^*$ , $p \neq 2$

[38]: `D = DD(1,1,2,2,3)`  
`GD = g.discriminant()(a2=p*a2d, a4=p^2*a4d, a6=p^3*a6d)`

We have  $\Delta \equiv 16\text{disc}(g) \pmod{p^7}$ :

[39]: `assert (D - 16*GD) % p^7 == 0`

Hence  $n \geq 6$ , with equality when  $p \neq 2$ .

##### 1.4.2 Type $I_0^*$ , $p = 2$

Now we have  $n \geq 8$ :

[40]: `D = DD(1,1,2,2,3, pr=2)`  
`GD = g.discriminant()(a2=2*a2d, a4=2^2*a4d, a6=2^3*a6d, p=2)`

We have  $\text{disc}(g) \equiv a_6^2 - a_2^2 a_4^2 = 2^6(a_6'^2 - a_2'^2 a_4'^2) \pmod{2^7}$ :

[41]: `assert (GD - 2^6*(a6d^2-a2d^2*a4d^2)) % 2^7 == 0`

Hence the condition that  $v(\text{disc}(g)) = 6$  is equivalent to  $a'_6 \not\equiv a'_2 a'_4 \pmod{2}$ , and so we can set  $a'_6 = a'_2 a'_4 + 2v + 1$ :

```
[42]: D = D(a6d=a2d*a4d+2*v+1)
```

Now  $\Delta \equiv a_1^4 a_4^2 - a_3^4 = 2^8 (a_1^4 a_4'^2 - a_3'^4) \pmod{2^9}$ :

```
[43]: assert (D-2^8*(a1d^4*a4d^2 - a3d^4)) % 2^9 == 0
```

Hence  $n \geq 8$ , with  $n = 8 \iff a'_3 \not\equiv a'_1 a'_4 \pmod{2}$ . Otherwise set  $a'_3 = a'_1 a'_4 + 2t$ :

```
[44]: D = D(a3d=a1d*a4d+2*t)
```

We have  $\Delta \equiv 2^8 a_1 = 2^9 a'_1 \pmod{2^{10}}$  (considering  $a'_4$  even/odd separately):

```
[45]: assert all(((D(a4d=2*w+r)-2^9*a1d^6)%2^10 ==0) for r in [0,1])
```

Hence  $n \geq 9$ , with  $n = 9$  if and only if  $a'_1$  is odd. Otherwise, assume  $v(a_1) \geq 2$ , so also  $v(a_3) \geq 3$  (keeping the condition that  $a'_6 \not\equiv a'_2 a'_4 \pmod{2}$ ):

```
[46]: D = DD(2,1,3,2,3, pr=2)(a6d=a2d*a4d+2*v+1)
```

Now we have  $\Delta \equiv 2^{10} \pmod{2^{11}}$ , so  $n = 10$ :

```
[47]: assert (D-2^10) % 2^11 == 0
```

In summary,  $n = 8, 9, 10$  with relative probabilities  $1/2, 1/4, 1/4$ .

## 1.5 Type IV\*, $W(1, 2, 2, 3, 4)$ with $v(b_6) = 4$

### 1.5.1 Type IV\*, $p \neq 3$

```
[48]: D = DD(1,2,2,3,4)
      B6 = BB6(1,2,2,3,4)
```

We have  $\Delta \equiv -3^3 b_6^2 \pmod{p^9}$ , so  $n \geq 8$  and  $n = 8$  for  $p \neq 3$ :

```
[49]: assert (D + 27*B6^2) % p^9 == 0
```

### 1.5.2 Type IV\*, $p = 3$

```
[50]: D = DD(1,2,2,3,4, pr=3)
      B4 = BB4(1,2,2,3,4, pr=3)
      B2 = BB2(1,2,2,3,4, pr=3)
```

We have  $v(b_2) \geq 2$ ,  $v(b_4) \geq 3$ , and  $\Delta \equiv b_4^3 \pmod{3^{10}}$ :

```
[51]: assert B2 % 3^2 == 0 and B4%3^3 ==0 and (D-B4^3) % 3^10 == 0
```

So  $n \geq 9$ , with  $n = 9 \iff v(b_4) = 3$ . Now  $v(b_4) \geq 4 \iff a'_1 a'_3 \equiv a'_4 \pmod{3}$ , which we can impose by setting  $a'_4 = a'_1 a'_3 + 3t$ :

```
[52]: D = D(a4d=a1d*a3d+3*t)
      B2 = BB2(1,2,2,3,4, pr=3)(a4d=a1d*a3d+3*t)
      B6 = BB6(1,2,2,3,4, pr=3)(a4d=a1d*a3d+3*t)
```

Now we have  $\Delta \equiv -3^4 b_2 b_6 \pmod{3^{10}}$ :

```
[53]: assert (D + 3^4*B2*B6) % 3^10 == 0
```

Hence  $n \geq 10$ , with  $n = 10 \iff v(b_2) = 2 \iff 2 \nmid a_1'^2 + a_2'$ . Otherwise, set  $a_2' = -a_1'^2 + 3u$ ; now,  $\Delta \equiv -3^3 b_6^2 \pmod{3^{12}}$ , so  $n = 11$  exactly:

```
[54]: D = D(a2d=3*u-a1d^2)
      assert (D+3^3*B6^2) % 3^12 == 0
```

In summary, we have  $n = 9, 10, 11$  with relative probabilities  $2/3, 2/9, 1/9$ .

## 1.6 Type III\*, $W(1, 2, 3, 3, 5)$

The exit condition is  $v(a_4) = 3$ .

### 1.6.1 Type III\*, $p \neq 2$

```
[55]: D = DD(1,2,3,3,5)
```

Now  $\Delta \equiv -2^6 p^9 a_4'^3 = -2^6 a_4^3 \pmod{p^{10}}$ :

```
[56]: assert (D+2^6*p^9*a4d^3) % p^10 ==0
```

Hence for  $p \neq 2$ , when the exit condition holds, we have  $n = 9$ .

### 1.6.2 Type III\*, $p = 2$

```
[57]: D = DD(1,2,3,3,5, pr=2)
```

Here,  $\Delta \equiv 2^{10} a_1^4 a_4'^2 \equiv a_1^4 a_4^2 \pmod{2^{11}}$ :

```
[58]: assert (D - 2^10*a1d^4*a4d^2) % 2^11 == 0
```

Hence  $n \geq 10$ ; when the exit condition  $v(a_4) = 3$  holds we have with  $n = 10 \iff 2 \nmid a_1' \iff v(a_1) = 1$ .

Assume that  $v(a_1) \geq 2$ :

```
[59]: D = DD(2,2,3,3,5, pr=2)
```

Now  $\Delta \equiv 2^{12} a_3^4 \equiv a_3^4 \pmod{2^{13}}$ :

[60]: `assert (D - 2^12*a3d^4) % 2^13 == 0`

Hence we have  $n \geq 12$ , with  $n = 12 \iff 2 \nmid a'_3 \iff v(a_3) = 3$ .

Assume that  $v(a_3) \geq 4$ :

[61]: `D = DD(2,2,4,3,5, pr=2)`

We have  $\Delta \equiv 2^{14}(a_4'^2(a_1'^4 + a_2'^2) + a_6'^2) \equiv 2^{14}(a_1'^4 + a_2'^2 + a_6'^2) \equiv 2^4(2^2a_1^4 + 2^6a_2^2 + a_6^2) \pmod{2^{15}}$ :

[62]: `assert (D - 2^14 * (a4d^2*(a1d^4 + a2d^2) + a6d^2)) % 2^15 == 0`

Hence  $n \geq 14$ , with  $n = 14 \iff 2 \nmid a'_1 + a'_2 + a'_6$ .

Setting  $a'_6 = a'_1 + a'_2 + 2t$ , consider the cases  $a'_1$  even/odd separately to see that  $\Delta \equiv 2^{15} \pmod{2^{16}}$  in both cases, so  $n = 15$ :

[63]: `D = D(a4d=2*u+1, a6d=a1d+a2d+2*t)`  
`assert all(((D(a1d=2*w+r)+2^15)%2^16)==0 for r in (0,1))`

In summary we have  $n = 10, 12, 14, 15$  with relative probabilities  $1/2, 1/4, 1/8, 1/8$  respectively.

## 1.7 Type II\*, $W(1, 2, 3, 4, 5)$

The exit condition is  $v(a_6) = 5$ .

**Type II\*,  $p \geq 5$**

[64]: `D = DD(1,2,3,4,5)`

Now  $n \geq 10$ , with equality for  $p \neq 2, 3$ , since  $\Delta \equiv -2^4 3^3 p^{10} a_6'^2 \equiv -2^4 3^3 a_6^2 \pmod{p^{11}}$ :

[65]: `assert (D + 2^4*3^3*p^10*a6d^2) % p^11 == 0`

### 1.7.1 Type II\*, $p = 3$

[66]: `D = DD(1,2,3,4,5, pr=3)`  
`B2 = BB2(1,2,3,4,5, pr=3)`  
`B4 = BB4(1,2,3,4,5, pr=3)`

We have  $v(b_2) \geq 2$ :

[67]: `assert B2%3^2 == 0`

Also,  $\Delta \equiv -a_6 b_2^3 = -3^5 a_6' b_2^3 \pmod{3^{12}}$ :

[68]: `assert ((D + 3^5*B2^3*a6d)%3^12) == 0`

Hence  $n \geq 11$ , and  $n = 11 \iff v(b_2) = 2 \iff 3 \nmid a_1'^2 + a_2'$ . Set  $a_2' = -a_1'^2 + 3t$ .

[69]: `D = D(a2d=-a1d^2+3*t)`  
`B4 = B4(a2d=-a1d^2+3*t)`

Now  $\Delta \equiv b_4^3 \pmod{3^{13}}$ , so  $n \geq 12$ , with  $n = 12 \iff v(b_4) = 3$ :

[70]: `assert (D-B4^3)%3^13 == 0`

We have  $v(b_4) \geq 4 \iff a'_1 a'_3 \equiv a'_4 \pmod{3}$ ; set  $a'_4 = a'_1 a'_3 + 3u$ :

[71]: `D = D(a4d=a1d*a3d+3*u)`

Now  $\Delta \equiv -3^3 a_6 = -3^{13} a_6^2 \pmod{3^{14}}$ , so  $n = 13$  exactly:

[72]: `assert (D+3^13*a6d^2)%3^14 == 0`

### 1.7.2 Type II\*, $p = 2$

[73]: `D = DD(1,2,3,4,5, pr=2)`

Now  $\Delta \equiv 2^{11} a_1^6 a_6' \equiv a_1^6 a_6 \pmod{2^{12}}$ :

[74]: `assert (D - 2^11*a1d^6*a6d) % 2^12 == 0`

So  $n \geq 11$ , with  $n = 11 \iff 2 \nmid a_1' \iff v(a_1) = 1$ . Assume  $v(a_1) \geq 2$ :

[75]: `D = DD(2,2,3,4,5, pr=2)`

Now  $\Delta \equiv a_3^4 = 2^{12} a_3'^4 \pmod{2^{13}}$ :

[76]: `assert (D - 2^12*a3d^4) % 2^13 == 0`

So  $n \geq 12$ , with  $n = 12 \iff 2 \nmid a_3' \iff v(a_3) = 3$ . Assume  $v(a_3) \geq 4$ :

[77]: `D = DD(2,2,4,4,5, pr=2) (a6d=2*u+1)`

Now  $n = 14$  exactly, since  $\Delta \equiv 2^{14} \pmod{2^{15}}$ :

[78]: `assert (D - 2^14) % 2^15 == 0`

In summary,  $n = 11, 12, 14$  with relative probabilities  $1/2, 1/4, 1/4$  respectively.

### 1.8 Type I\*\_m ( $m \geq 1$ ), $W(1, = 1, 2, 3, 4)$

In order to impose the condition  $(a_1, a_2, a_3, a_4, a_6) \in W_{\text{odd}}(k) = W(1, = 1, k+1, k+2, 2k+2)$  or  $W_{\text{even}}(k) = W(1, = 1, k+2, k+2, 2k+3)$  for  $k \geq 1$ , we use the variable  $q$  to denote a fixed power of  $p$  depending on  $k$ .

### 1.8.1 Type $I_m^*$ , $p \neq 2$

First consider  $m = 2k - 1 \geq 1$  with  $k \geq 1$ , where we want to show that  $n = v(\Delta) = m + 6 = 2k + 5$ . Since  $k \geq 1$ , we take  $q = p^{k-1}$ , so  $v(q) = k - 1 \geq 0$ . Then  $p \mid a_1, a_2, p^2q \mid a_3, p^3q \mid a_4$ , and  $p^4q^2 \mid a_6$ . The exit condition is  $v(b_6) = 2k + 2 = v(p^4q^2)$ .

```
[79]: D = Delta(a1=p*a1d, a2=p*a2d, a3=p^2*q*a3d, a4=p^3*q*a4d, a6=p^4*q^2*a6d)
      B6 = b6(a1=p*a1d, a2=p*a2d, a3=p^2*q*a3d, a4=p^3*q*a4d, a6=p^4*q^2*a6d)
```

We have  $\Delta \equiv -2^4p^3a_2^3b_6 \pmod{p^8q^2 = p^{2k+6}}$ :

```
[80]: assert (D + 2^4*p^3*a2d^3*B6) % (p^8*q^2) == 0
```

Since  $p \nmid a_2'$ , and  $v(b_6) = 2k + 2$ , for  $p \neq 2$  we have  $n = 2k + 5$  exactly.

Now consider  $m = 2k \geq 2$ , with  $k \geq 1$ , where we want to show that  $n = m + 6 = 2k + 6$ . Again with  $q = p^{k-1}$ , we now have  $p \mid a_1, a_2, p^3q \mid a_3, a_4$ , and  $p^5q^2 \mid a_6$ . The exit condition is now  $v(b_8) = 2k + 4 = v(p^6q^2)$ .

```
[81]: D = Delta(a1=p*a1d, a2=p*a2d, a3=p^3*q*a3d, a4=p^3*q*a4d, a6=p^5*q^2*a6d)
      B8 = b8(a1=p*a1d, a2=p*a2d, a3=p^3*q*a3d, a4=p^3*q*a4d, a6=p^5*q^2*a6d)
```

Now  $\Delta \equiv -2^4p^2b_8a_2'^2 \pmod{p^9q^2 = p^{2k+7}}$ :

```
[82]: assert (D + 2^4*p^2*B8*a2d^2) % (p^9*q^2) == 0
```

Since  $v(2^4p^2b_8a_2'^2) = 2 + v(b_8) = 2k + 6$ , we have  $n = 2k + 6$  exactly.

### 1.8.2 Type $I_m^*$ , $p = 2$

#### 1.8.3 $p = 2, m = 1$ : $W(1, = 1, 2, 3, 4)$

For  $m = 2k - 1 = 1$ , we are in  $W_{\text{odd}}(1)$  with exit condition  $v(a_3) = k + 1 = 2$ :

```
[83]: D = DD(1,1,2,3,4, pr=2)(a2d=2*t+1)
```

We have  $\Delta \equiv 2^8a_3^4 \pmod{2^9}$ :

```
[84]: assert (D - 2^8*a3d^4) % 2^9 == 0
```

Hence the exit condition implies that  $n = 8$ .

#### 1.8.4 $p = 2, m = 2$ : $W(1, = 1, 3, 3, 5)$

Now  $m = 2k = 2$  and the exit condition is  $v(a_4) = k + 2 = 3$ :

```
[85]: D = DD(1,1,3,3,5, pr=2)(a2d=2*t+1)
```

We have  $\Delta \equiv 2^{10}a_1^4a_4^2 \pmod{2^{11}}$ :

```
[86]: assert (D - 2^10*a1d^4*a4d^2) % 2^11 == 0
```



**1.8.7**  $p = 2$ ,  $m = 2k - 1 \geq 5$  with  $k \geq 3$ ,  $W_{\text{odd}}(k) = W(1, = 1, k + 1, k + 2, 2k + 2)$

Since  $k \geq 3$ , we now take  $q = 2^{k-3}$ , so  $v(q) = k - 3 \geq 0$ . Then  $2 \mid a_1, a_2, 2^4q \mid a_3, 2^5q \mid a_4$ , and  $2^8q^2 \mid a_6$ .

Here,  $v(a_3) = k + 1$  is the exit condition.

```
[97]: D = Delta(a1=2*a1d, a2=2*a2d, a3=2^4*q*a3d, a4=2^5*q*a4d, a6=2^8*q^2*a6d,
↳p=2)(a2d=2*t+1) #, a3d=2*u+1)
```

We have  $\Delta \equiv 2^{13}q^2a_1'^4a_3'^2 = 2^{2k+7}a_1'^4a_3'^2 \pmod{2^{14}q^2 = 2^{2k+8}}$ :

```
[98]: assert (D-2^13*q^2*a1d^4*a3d^2) % (2^14*q^2) == 0
```

Hence  $n \geq 2k + 7$ , and, assuming the exit condition  $v(a_3') = 0$ , we have  $n = 2k + 7 \iff 2 \nmid v(a_1') \iff v(a_1) = 1$ . Assume that  $v(a_1) \geq 2$ :

```
[99]: D = Delta(a1=4*a1d, a2=2*a2d, a3=2^4*q*a3d, a4=2^5*q*a4d, a6=2^8*q^2*a6d,
↳p=2)(a2d=2*t+1, a3d=2*u+1)
```

Now we have  $\Delta \equiv 2^{15}q^2 = 2^{2k+9} \pmod{2^{16}q^2 = 2^{2k+10}}$ , so  $n = 2k + 9$ :

```
[100]: assert (D-2^15*q^2) % (2^16*q^2) == 0
```
